# Supplementary material for: Consensus of Consensus: Decentralized Consensus-Based Optimization
Source: arXiv:2611.27433 source file (2026-11-20)
Supplement: Supplementary file 1 [file supplement_SIAM.tex]

% SIAM Supplemental File Template
\documentclass[review,supplement,hidelinks,onefignum,onetabnum]{siam/siamart251216}

\input{siam/shared}

\externaldocument[][nocite]{main_SIAM}

% Optional PDF information
\ifpdf
\hypersetup{
}
\fi

\begin{document}
\maketitle

\input{ballet}

\bibliographystyle{siam/siamplain}
\bibliography{references}


\end{document}
